# Supplementary material for: ROAST: Review-level Opinion Aspect Sentiment Target Joint Detection for ABSA
Source: arXiv:2405.20274 source file (2024-07-18)
Supplement: Supplementary file 1 [file 9-Appendix.tex]

\begin{table*}[!ht]
        \centering
        \caption{Example Reviews and label Quadruples for all the domains and languages}
        \label{tab: reviews-quads}
        \resizebox{\textwidth}{!}{%
        \begin{tabular}{|p{2cm}|p{10cm}|p{13cm}|}
        \hline
        \begin{tabular}[c]{@{}p{2cm}@{}}\textbf{Dataset, Lang, \& Source} \end{tabular} &
          \begin{tabular}[r]{@{}c@{}} \textbf{Example Review} \end{tabular} &
          \begin{tabular}[r]{@{}c@{}} \textbf{Quadruples} \end{tabular} \\ \hline
        \begin{tabular}[c]{@{}p{2cm}@{}}
            Amazon\_FF \\\\ English \\\\ \href{https://www.kaggle.com/snap/amazon-fine-food-reviews}{Kaggle Amazon Fine Foods Data}
        \end{tabular} 
        &
          \begin{tabular}[c]{@{}p{10cm}@{}}I live in the area where these cookies are made, and I remember buying them from local coffee stands when they first started making them years ago - - each one was wrapped in saran wrap and had a handwritten label on them. The packaging has changed, and there are many different flavors available now, but the original breakfast cookie still tastes just as good today as those first ones did. The smaller size is great for a snack, as the large ones are enough for two people! Full of good stuff, not too sweet. It's a treat that you can feel good about .\end{tabular} &
          \begin{tabular}[c]{@{}p{13cm}@{}} {[}{[}'food style\_options', 'cookies', 'many different flavors available', 'positive'{]}, \\ {[}'food quality', 'cookies', 'original breakfast cookie still tastes just as good', 'positive'{]}, \\ {[}'food style\_options', 'cookies', 'smaller size is great for a snack', 'positive'{]}, \\ {[}'food style\_options', 'cookies', 'large ones are enough for two people', 'positive'{]}, \\ {[}'shipment quality', 'NULL', 'packaging has changed', 'positive'{]}, \\ {[}'food general', 'cookies', 'Full of good stuff', 'positive'{]}, \\ {[}'food quality', 'cookies', 'not too sweet', 'positive'{]}, \\ {[}'food general', 'cookies', 'treat that you can feel good about', 'positive'{]}{]}\end{tabular} \\ \hline
        \begin{tabular}[c]{@{}p{2cm}@{}}
          Coursera \\\\ English \\\\ \href{https://www.kaggle.com/datasets/septa97/100k-courseras-course-reviews-dataset}{Kaggle Coursera Course Dataset}\\
        \end{tabular} 
        &
          \begin{tabular}[c]{@{}p{10cm}@{}}Andrew Ng teaches a great Machine Learning course . Ng speaks clearly, and the flow of the class is easy to follow. The examples made things clear and the homework exercises really cemented the learning points. Overall, the class was just the right amount of challenge and fun. I now have a solid understanding and intuition about Machine Learning and will use what I've learned.  Thank you Andrew Ng !\end{tabular} &
          \begin{tabular}[c]{@{}p{13cm}@{}}{[}{[}'course general', 'Machine Learning course', 'great', 'positive'{]}, \\ {[}'faculty comprehensiveness', 'Andrew Ng', 'speaks clearly', 'positive'{]}, \\ {[}'material comprehensiveness', 'examples', 'made things clear', 'positive'{]}, \\ {[}'assignments comprehensiveness', 'homework exercises', 'cemented the learning points', 'positive'{]}, \\ {[}'course general', 'class', 'just the right amount of challenge and fun', 'positive'{]}, \\ {[}'course comprehensiveness', 'Machine Learning course', 'solid understanding and intuition', 'positive'{]}, \\ {[}'faculty general', 'Andrew Ng', 'Thank you', 'positive'{]}, \\ {[}'faculty comprehensiveness', 'Andrew Ng', 'flow of the class is easy to follow', 'positive'{]}{]}\end{tabular} \\ \hline
        \begin{tabular}[c]{@{}p{2cm}@{}}
          \\Hotels \\\\ English \\\\ \citet{TripAdvisor-dataset}\\
        \end{tabular} 
        &
          \begin{tabular}[c]{@{}p{10cm}@{}}Pleasantly surprised Very close to airport, staff kindly checked me in very early and after I freshened up pointed me in the right direction to the main centre. here is a 4 storey outlet mall attached and MTR right next door. 20minutes and in Kowloon. Room was unexpectedly ample, well fitted out and great value.\end{tabular} &
          \begin{tabular}[c]{@{}p{13cm}@{}}{[}{[}'hotel general', 'NULL', 'Pleasantly surprised', 'positive'{]}, \\ {[}'location general', 'NULL', 'Very close to airport', 'positive'{]}, \\ {[}'service general', 'staff', 'kindly checked me in very early', 'positive'{]}, \\ {[}'location general', 'NULL', '4 storey outlet mall attached', 'positive'{]}, \\ {[}'location general', 'NULL', 'MTR right next door', 'positive'{]}, \\ {[}'location general', 'NULL', '20minutes and in Kowloon', 'positive'{]}, \\ {[}'rooms design\_features', 'Room', 'unexpectedly ample', 'positive'{]}, \\ {[}'rooms general', 'Room', 'well fitted', 'positive'{]}, \\ {[}'rooms prices', 'Room', 'great value', 'positive'{]}{]}\end{tabular} \\ \hline
        \multirow{2}{*}{\begin{tabular}[c]{@{}p{2cm}@{}}
          Phones \\\\ Hindi \\ English \\\\ \href{www.amazon.in}{amazon.in}\\ \href{https://hindi.gadgets360.com}{Gadgets360} \\ \href{https://hindi.gizbot.com}{Gizbot} \\ \href{https://www.jansatta.com}{IndianExpress}
        \end{tabular}} 
        &
          \begin{tabular}[c]{@{}p{10cm}@{}}Worst worst top worst product i bought from realme . i got so annoyed . speed is much much worse one . realme and amazon must pay back my money . all the time the mobile is sleeping . once u got call , we need to wakeup the mobile\end{tabular} &
          \begin{tabular}[c]{@{}p{13cm}@{}}{[}{[}'product', 'phone general', 'negative', 'Worst'{]}, \\ {[}'product', 'phone general', 'negative', 'worst'{]}, \\ {[}'product', 'phone general', 'negative', 'top worst'{]}, \\ {[}'product', 'phone general', 'negative', 'so annoyed'{]}, \\ {[}'product', 'phone operation\_performance', 'negative', 'speed is much much worse'{]}, \\ {[}'product', 'phone general', 'negative', 'sleeping'{]}\end{tabular} \\ \cline{2-3}
        % \begin{tabular}[c]{@{}p{2cm}@{}}
        %     Phones\\\\ Hindi\\\\ \href{www.amazon.in}{amazon.in}\\ \href{https://hindi.gadgets360.com}{Gadgets360} \\ \href{https://hindi.gizbot.com}{Gizbot} \\ \href{https://www.jansatta.com}{IndianExpress}
        % \end{tabular} 
        &
        \begin{tabular}[c]{@{}p{10cm}@{}} \\
          \foreignlanguage{hindi}{15 मिनट में उपयोग के दौरान हीटिंग की समस्या। टच स्क्रीन कभी-कभी जारी करती है यह बहुत बढ़िया है और कभी-कभी आपको टाइप करते समय सैमसंग कुंजी पैड पर भी कई बार स्पर्श करना पड़ता है। हम सभी परिवार सैमसंग मोबाइल का उपयोग कर रहे हैं लेकिन इस बार मैं मुद्दों से चिंतित हूं | अगर मुझे समान मुद्दों का सामना करना पड़ता है तो मुझे मोबाइल बदलना होगा और डेटा ट्रांसफर करना होगा यह बहुत परेशान करने वाला काम है | अगर कोई सैमसंग इस समीक्षा को पढ़ रहा है तो कृपया मुझे अमेज़ॅन के माध्यम से उत्तर दें .}
        \end{tabular} &   
        \begin{tabular}[c]{@{}p{13cm}@{}}
            {[}
                {[}'Phone Quality', \foreignlanguage{hindi}{'सैमसंग', 'हीटिंग की समस्या'}, 'Negative'{]}, \\
                {[}'Display Quality', \foreignlanguage{hindi}{'टच स्क्रीन', 'कई बार स्पर्श करना पड़ता है'}, 'Negative'{]},\\
                {[}'Phone General', \foreignlanguage{hindi}{'सैमसंग', 'मुद्दों से चिंतित हूं'}, 'Negative'{]},\\
                {[}'Phone General', \foreignlanguage{hindi}{'सैमसंग', 'बहुत परेशान करने वाला काम है'}, 'Negative'{]}
            {]}
        \end{tabular}
        \\ \hline
        \begin{tabular}[c]{@{}p{2cm}@{}}
            Movies \\\\ Telugu\\\\ \href{http://www.123telugu.com/}{123telugu}
        \end{tabular} &
          \begin{tabular}[c]{@{}p{10cm}@{}}\foreignlanguage{telugu}{మొత్తంగా చెప్పాలంటే  ఏజెంట్ సాయి శ్రీనివాస ఆత్రేయ ఆసక్తి కరమైన కథనంతో సాగే ఉత్కంఠ రేపే ఓ మంచి కామెడీ థ్రిల్లర్. ఆకట్టుకునే నటనతో పాటు, మంచి డైలాగ్ డిక్షన్ తో  నవీన్ పోలిశెట్టి హీరోగా తన మొదటి సినిమాతోనే మంచి ప్రభావం చూపాడు.  వాస్తవికతకు దగ్గరగా ఉండే ఆసక్తికరమైన కథనం ప్రేక్షకుడిని సినిమాలో లీనమయ్యేలా చేస్తుంది. చివరి 10నిమిషాలు మినహాయించి, ప్రేక్షకుడికి కావలసిన అన్ని ఎలిమెంట్స్ ఈ చిత్రంలో ఉన్నాయి. ఈ వారాంతపు సెలవులు ఓ మంచి మూవీతో ముగించాలనుకునే వారికి ఏజెంట్ సాయి శ్రీనివాస ఆత్రేయ మూవీ బెస్ట్ చాయిస్ అనడంలో ఎటువంటి సందేహం లేదు.}\end{tabular} &
          \begin{tabular}[c]{@{}p{13cm}@{}}
              {[}
                  {[}'movie general', '\foreignlanguage{telugu}{ఏజెంట్ సాయి శ్రీనివాస ఆత్రేయ}', '\foreignlanguage{telugu}{మంచి కామెడీ థ్రిల్లర్}', 'positive'{]},\\ 
                  {[}'story quality', '\foreignlanguage{telugu}{కథనంతో}', '\foreignlanguage{telugu}{ఆసక్తి కరమైన}', 'positive'{]}, \\
                  {[}'movie general', '\foreignlanguage{telugu}{ఏజెంట్ సాయి శ్రీనివాస ఆత్రేయ}', '\foreignlanguage{telugu}{ఉత్కంఠ రేపే}', 'positive'{]}, \\
                  {[}'actor action', '\foreignlanguage{telugu}{నవీన్ పోలిశెట్టి}', '\foreignlanguage{telugu}{ఆకట్టుకునే నటనతో}', 'positive'{]},\\
                  {[}'actor dialogues', '\foreignlanguage{telugu}{నవీన్ పోలిశెట్టి}', '\foreignlanguage{telugu}{మంచి డైలాగ్ డిక్షన్}', 'positive'{]},\\
                  {[}'actor general', '\foreignlanguage{telugu}{నవీన్ పోలిశెట్టి}', '\foreignlanguage{telugu}{మంచి ప్రభావం చూపాడు}', 'positive'{]},\\
                  {[}'story engagement', '\foreignlanguage{telugu}{కథనం}', '\foreignlanguage{telugu}{వాస్తవికతకు దగ్గరగా ఉండే}', 'positive'{]},\\
                  {[}'story quality', '\foreignlanguage{telugu}{కథనం}', '\foreignlanguage{telugu}{ఆసక్తికరమైన}', 'positive'{]},\\
                  {[}'story engagement', '\foreignlanguage{telugu}{కథనం}', '\foreignlanguage{telugu}{ప్రేక్షకుడిని సినిమాలో లీనమయ్యేలా చేస్తుంది}', 'positive'{]},\\
                  {[}'movie general', '\foreignlanguage{telugu}{ఏజెంట్ సాయి శ్రీనివాస ఆత్రేయ}', '\foreignlanguage{telugu}{అన్ని ఎలిమెంట్స్ ఈ చిత్రంలో ఉన్నాయి}', 'positive'{]},\\
                  {[}'movie general', '\foreignlanguage{telugu}{ఏజెంట్ సాయి శ్రీనివాస ఆత్రేయ}', '\foreignlanguage{telugu}{మంచి మూవీ}', 'positive'{]},\\
                  {[}'movie general', '\foreignlanguage{telugu}{ఏజెంట్ సాయి శ్రీనివాస ఆత్రేయ}', '\foreignlanguage{telugu}{బెస్ట్ చాయిస్}', 'positive'{]}
              {]}
                      \end{tabular}  \\ \hline
        \end{tabular}%
        }
    \end{table*}
